# Supplementary material for: DLME: Deep Local-flatness Manifold Embedding
Source: arXiv:2207.03160 source file (2022-07-26)
Supplement: Supplementary file 1 [file Sec_appendix_proof_1.tex]

\subsection{Details of Eq. (\ref{eq:lemma1})}
\label{app_proof_1}

\ 

\noindent \textbf{Eq. (\ref{eq:lemma1})}.
Let network $g_\phi(\cdot)$ to be Lipschitz continuity mapping. $d^z_{ij} = k^* d^y_{ij} , k^* \in [1/K, K]$, where $K$ is a Lipschitz constant. For neighborhoods points $i$ and $j$, The difference between DLME loss $L_{\text{D}}$ and contrastive learning loss $L_c$ is 
\begin{equation}
  \begin{aligned}
    |L_{\text{D}}\!-\! L_\text{c}| = 
    \mathbb{E}_{\substack{x_j, x_j }} 
      \left[
        A_{ij} 
        \!-\!
        \kappa \left((1\!+\!(\alpha\!-\!1)A_{ij}) k^* d^z_{ij} \right)
      \log
      (
        % \frac
        %   {1}
        {\frac{1}{\kappa\!(\! d_{ij}^{z}\!)}}
        \!-\!
        1
      )
      \right],
  \end{aligned}
  \label{eq:appendix_lemma1}
\end{equation}

\textbf{Detail.}
The contrastive learning loss is written as, For notational simplicity, we omit redundant symbols:
\begin{equation}
  \begin{aligned}
    L_c \!
    &= \! \mathbb{E}_{
      \substack{x_j, x_j }
      }
      \left[ 
        B_{ij}
        \log 
        \kappa \left(d_{ij}^{e}, \nu\right)
        +
        \left(1-B_{ij} \right)
        \log 
        \left(1-\kappa \left(d_{ij}^{e}, \nu \right) \right)
      \right] 
      \\
    \!&= \! \mathbb{E}_{
        \substack{x_j, x_j}
        }
      \left[
        B_{ij}
        \log 
        \kappa \left(d_{ij}^{e}\right)
        +
        \left(1-B_{ij}\right)
        \log 
        \left(
          1-\kappa \left(d_{ij}^{e}\right)
        \right)
      \right]
  \end{aligned}
\end{equation}
where $B_{ij}  = \pi[(x_i, x_j)\!\in\! E]$ shows weath $i$ and $j$ are neighborhoods in graph $G(X,E)$.

the DLME loss is written as, we :
\begin{equation}
    \begin{aligned}
      L_{\text{D}} & 
      \!=\! 
      E_{\substack{ x_i, x_j}} 
      \left[ 
        \mathcal{D}
        \left(
          \kappa 
          \left(
            R_{ij}  d^y_{ij}, \nu 
          \right)
          ,
          \kappa 
          \left( d^z_{ij},\nu \right)
        \right)
      \right] 
      \\
      \!&=\! E_{\substack{x_i, x_j}} 
      \left[ 
        \mathcal{D}\left(
            \kappa \left(
              R_{ij}  d^y_{ij} 
              \right)
          , \kappa \left( d^z_{ij} \right)
            \right)
      \right]
    \end{aligned}
    \label{eq:appendix_dlme}
\end{equation}

We substitute Eq. (\ref{eq:D}) into Eq. (\ref{eq:appendix_dlme}).

\begin{equation}
    \begin{aligned}
      L_{\text{D}} & \!= 
      \! E_{
        \substack{ 
            x_i, x_j   
            }    
        } 
        \left[
            \kappa \left(R_{ij}  d^y_{ij}  \right) 
            \log 
            \kappa \left( d^z_{ij} \right) 
            + 
            \left(1-\kappa \left(R_{ij}  d^y_{ij}  \right)\right)
            \log
            \left(1-\kappa \left( d^z_{ij} \right)\right)
        \right]
      \\
    \end{aligned}
    \label{eq:appendix_dlme}
\end{equation}

% We assume that network $g_\phi(\cdot)$ to be Distance-preserving mapping, then

% \begin{equation}
%     d^y_{ij} = d^z_{ij}
% \end{equation}

% and 

% \begin{equation}
%     \begin{aligned}
%       L_{\text{D}} & \!= 
%       \! E_{
%         \substack{ 
%             x_i, x_j   
%             }    
%         } 
%         \left[
%             \kappa \left(R_{ij}  d^y_{ij}  \right) 
%             \log 
%             \kappa \left( d^y_{ij} \right) 
%             + 
%             \left(1-\kappa \left(R_{ij}  d^y_{ij}  \right)\right)
%             \log
%             \left(1-\kappa \left( d^y_{ij} \right)\right) 
%         \right]
%       \\
%     \end{aligned}
%     \label{eq:appendix_dlme}
% \end{equation}

The difference between the two loss functions is:

\begin{equation}
  \begin{aligned}
      &L_c - L_{\text{D}}\\
      =
      &\mathbb{E}_{\substack{x_j, x_j }}
      \left[ 
          % \left(
              B_{ij}
              \log \kappa \left( d_{ij}^{z}\right)
              +
              \left(1-B_{ij} \right)
              \log \left(1-\kappa \left(d_{ij}^{z}\right)\right)
          % \right)
      \right]
      - \\
      &\mathbb{E}_{\substack{x_j, x_j }}
      \left[
          % \left(
              \kappa \left(R_{ij}  d^y_{ij}  \right) 
              \log \kappa \left( d^z_{ij} \right) 
              + 
              \left(1-\kappa \left(R_{ij} d^y_{ij} \right)\right)
              \log \left(1-\kappa \left( d^z_{ij} \right)\right) 
          % \right)
      \right]\\
%     \end{aligned}
%     \label{eq:appendix_diff_twoloss_2}
% \end{equation}
% \begin{equation}
%   \begin{aligned}
    % &L_c-L_{\text{D}} \\
    =
    &\mathbb{E}_{\substack{x_j, x_j }}
    \!\biggl[\! 
      B_{ij}
      \log \kappa \!\left(\! d_{ij}^{z}\!\right)\!
      \!+\!
      \left(1\!-\!B_{ij} \right)
      \log \!\left(\!1-\kappa \left(d_{ij}^{z}\right)\!\right)\!
      \!-\! 
      \kappa \left(R_{ij}d^y_{ij} \right) 
      \log \kappa \left( d^z_{ij} \right) 
      \!-\! 
      \left(1\!-\!\kappa \left(R_{ij}  d^y_{ij}  \right)\right)
      \log \left(1\!-\!\kappa \left( d^z_{ij}\right)\right) 
    \!\biggl]\! \\
    =&\!\mathbb{E}_{\substack{x_j, x_j }}\biggl[\! 
      \left(
        B_{ij} - \kappa \left(R_{ij}d^y_{ij} \right)
      \right)
      \log \kappa \!\left(\! d_{ij}^{z}\!\right)\!
      +
      \left(
        1-B_{ij} -1 + \kappa \left( R_{ij} d^y_{ij} \right) 
      \right)
      \log \!\left(\!1-\kappa \left(R_{ij}  d^z_{ij}\right)\!\right)\!
    \!\biggl]\! \\
    =&\!\mathbb{E}_{\substack{x_j, x_j }}\biggl[\! 
      \left(
        B_{ij} - \kappa \left(R_{ij}d^y_{ij} \right)
      \right)
      \log \kappa \!\left(\! d_{ij}^{z}\!\right)\!
      +
      \left(
        \kappa \left( R_{ij} d^y_{ij} \right) - B_{ij}
      \right)
      \log \!\left(\!1-\kappa \left(d^z_{ij}\right)\!\right)\!
    \!\biggl]\! \\
    =&\!\mathbb{E}_{\substack{x_j, x_j }}\biggl[\! 
      \left(
        B_{ij} - \kappa \left(R_{ij}d^y_{ij} \right)
      \right)
      \left(
        \log \kappa \!\left(\! d_{ij}^{z}\!\right)\!
        -
        \log \!\left(\!1-\kappa \left(d^z_{ij}\right)\!\right)\!
      \right)
    \!\biggl]\! \\
    =&-\!\mathbb{E}_{\substack{x_j, x_j }}\biggl[\! 
      \left(
        B_{ij} - \kappa \left(R_{ij}d^y_{ij} \right)
      \right)
      \log
      \left(
        \frac
          {1-\kappa \left(d^z_{ij}\right)}
          {\kappa \!\left(\! d_{ij}^{z}\!\right)}
      \right)
    \!\biggl]\! \\
    =&-\!\mathbb{E}_{\substack{x_j, x_j }}\biggl[\! 
    \left(
      B_{ij} - \kappa \left(R_{ij}d^y_{ij} \right)
    \right)
    \log
    \left(
      \frac
        {1}
        {\kappa \!\left(\! d_{ij}^{z}\!\right)}
      -
      1
    \right)
  \!\biggl]\! \\
\end{aligned}
\label{eq:appendix_diff_twoloss_3}
\end{equation}

Substituting the relationship between $B_{ij}$ and $R_{ij}$, $R_{ij} = 1+(\alpha -1)B_{ij}$, we have

\begin{equation}
  \begin{aligned}
    L_c - L_{\text{D}}=-\!\mathbb{E}_{\substack{x_j, x_j }}
    \biggl[\! 
      \left(
        B_{ij} - \kappa \left((1+(\alpha -1)B_{ij})d^y_{ij} \right)
      \right)
      \log
      \left(
        \frac
          {1}
          {\kappa \!\left(\! d_{ij}^{z}\!\right)}
        -
        1
      \right)
    \!\biggl]\! \\
  \end{aligned}
\label{eq:appendix_diff_twoloss_3}
\end{equation}

We assume that network $g_\phi(\cdot)$ to be a Lipschitz continuity function, then

\begin{equation}
  \begin{aligned}
    \frac{1}{K} g_\phi(d^y_{ij}) \leq d^y_{ij} \leq K g_\phi(d^y_{ij}) \quad \forall i, j \in \{1,2,\cdots,N\}\\
    \frac{1}{K} d^z_{ij} \leq d^y_{ij} \leq K d^z_{ij} \quad \forall i, j \in \{1,2,\cdots,N\}
  \end{aligned}
\end{equation}

We construct the inverse mapping of $g_\phi(\cdot)$ : $g_\phi^{-1}(\cdot)$

\begin{equation}
  \begin{aligned}
    \frac{1}{K} d^z_{ij} \leq d^y_{ij} \leq K d^z_{ij} \quad \forall i, j \in \{1,2,\cdots,N\}
  \end{aligned}
\end{equation}

then exit $k^*$, let:
\begin{equation}
  \begin{aligned}
     d^y_{ij} = k^* d^z_{ij} \quad k^* \in [1/K, K] \quad \forall i, j \in \{1,2,\cdots,N\}
  \end{aligned}
  \label{eq:g_revers}
\end{equation}

Substituting the Eq.(\ref{eq:g_revers}) into Eq.(\ref{eq:appendix_diff_twoloss_3}).

\begin{equation}
  \begin{aligned}
    L_c - L_{\text{D}}=-\!\mathbb{E}_{\substack{x_j, x_j }}
    \biggl[\! 
      \left(
        B_{ij} - \kappa \left((1+(\alpha -1)B_{ij}) k^* d^z_{ij} \right)
      \right)
      \log
      \left(
        \frac
          {1}
          {\kappa \!\left(\! d_{ij}^{z}\!\right)}
        -
        1
      \right)
    \!\biggl]\! \\
  \end{aligned}
\label{eq:appendix_diff_twoloss_4}
\end{equation}

if $B_{ij}=1$, we have:  

\begin{equation}
  \begin{aligned}
  L_c - L_{\text{D}} \quad |_{B_{ij} =1} = -\!\mathbb{E}_{\substack{x_j, x_j }} 
  \biggl[
    \left(
      1 - \kappa \left(\alpha k^* d^z_{ij} \right)
    \right)
    \log
    \left(
      \frac
        {1}
        {\kappa \!\left(\! d_{ij}^{z}\!\right)}
      -
      1
    \right)
  \biggl] \\ 
  \end{aligned}
\end{equation}

then:

\begin{equation}
  \begin{aligned}
    &\lim_{\alpha \to 0} 
    L_c - L_{\text{D}} \quad |_{B_{ij} =1}
    \\
    = &-\!\mathbb{E}_{\substack{x_j, x_j }} 
  \biggl[
    \left(
      1 - \kappa \left(\alpha k^* d^z_{ij} \right)
    \right)
    \log
    \left(
      \frac
        {1}
        {\kappa \!\left(\! d_{ij}^{z}\!\right)}
      -
      1
    \right)
  \biggl] \\
  = & 0
  \end{aligned}
  \label{eq:lim}
\end{equation}

Based on Eq.(\ref{eq:lim}), we find that if $i,j$ is neighbor and $\alpha\to0$, there is no difference between the two loss functions $L_c$ and $L_{\text{D}}$.
When $\alpha \nrightarrow  0$,  the difference between the loss functions will be the function of $d_{ij}^{z}$. Because the contrastive learning loss $L_c$ only minimizes the distance between adjacent nodes and does not maintain any structural information. We believe that the loss of DLME will better preserve the structural information based on contrastive loss.
