# Supplementary material for: DLME: Deep Local-flatness Manifold Embedding
Source: arXiv:2207.03160 source file (2022-07-26)
Supplement: Supplementary file 2 [file Sec_appendix_proof_2.tex]

\clearpage

\subsection{Proof of Lemma 1}
\label{app_proof_2}

\ 
% \noindent \textbf{Lemma 2}.
% let $\kappa \left( d, \nu^y \right)$ and $\kappa \left( d, \nu^z \right)$ be two kernals function defined in Eq.(\ref{eq:t_dis}). when $\nu^z < \nu^y$, existing $d_p$, let $(d^y - d_p)(d-d^z_{ij})<0$, 
% then $ d^y_{ij} - d^z_{ij} > 0 $ and if $d_{ij}^y < {d_p}^y$ , 
% then $ d^y_{ij} - d^z_{ij} < 0 $.

% \noindent\fbox{
  % \parbox{0.99\textwidth}{
    \noindent \textbf{Lemma 1 (Push-pull property)}.
    let 
    % $\kappa \left( d, \nu^y \right)$ and $\kappa \left( d, \nu^z \right)$ be two kernals function.
    $\nu^y<\nu^z$
    and let $d^{z+} = \kappa^{-1}(\kappa(d, \nu^y), \nu^z)$ be the solution of minimizing $L_\text{D}$. 
    % Then exciting a threshold $d_p$,  if $d^y < d_p $, then $d^{z+} < d^y$ (shown in yellow in figure \ref{fig:FIg-dl}). And if $d^y > d_p $, then $d^{z+} > d^y$ (shown in pink).
    Then exists $d_p$ so that $(d^y - d_p) (d^{z+} - d^y) >0$.
  % }
% }

\begin{figure}[t]
  \centering
  \includegraphics[width=4.2in]{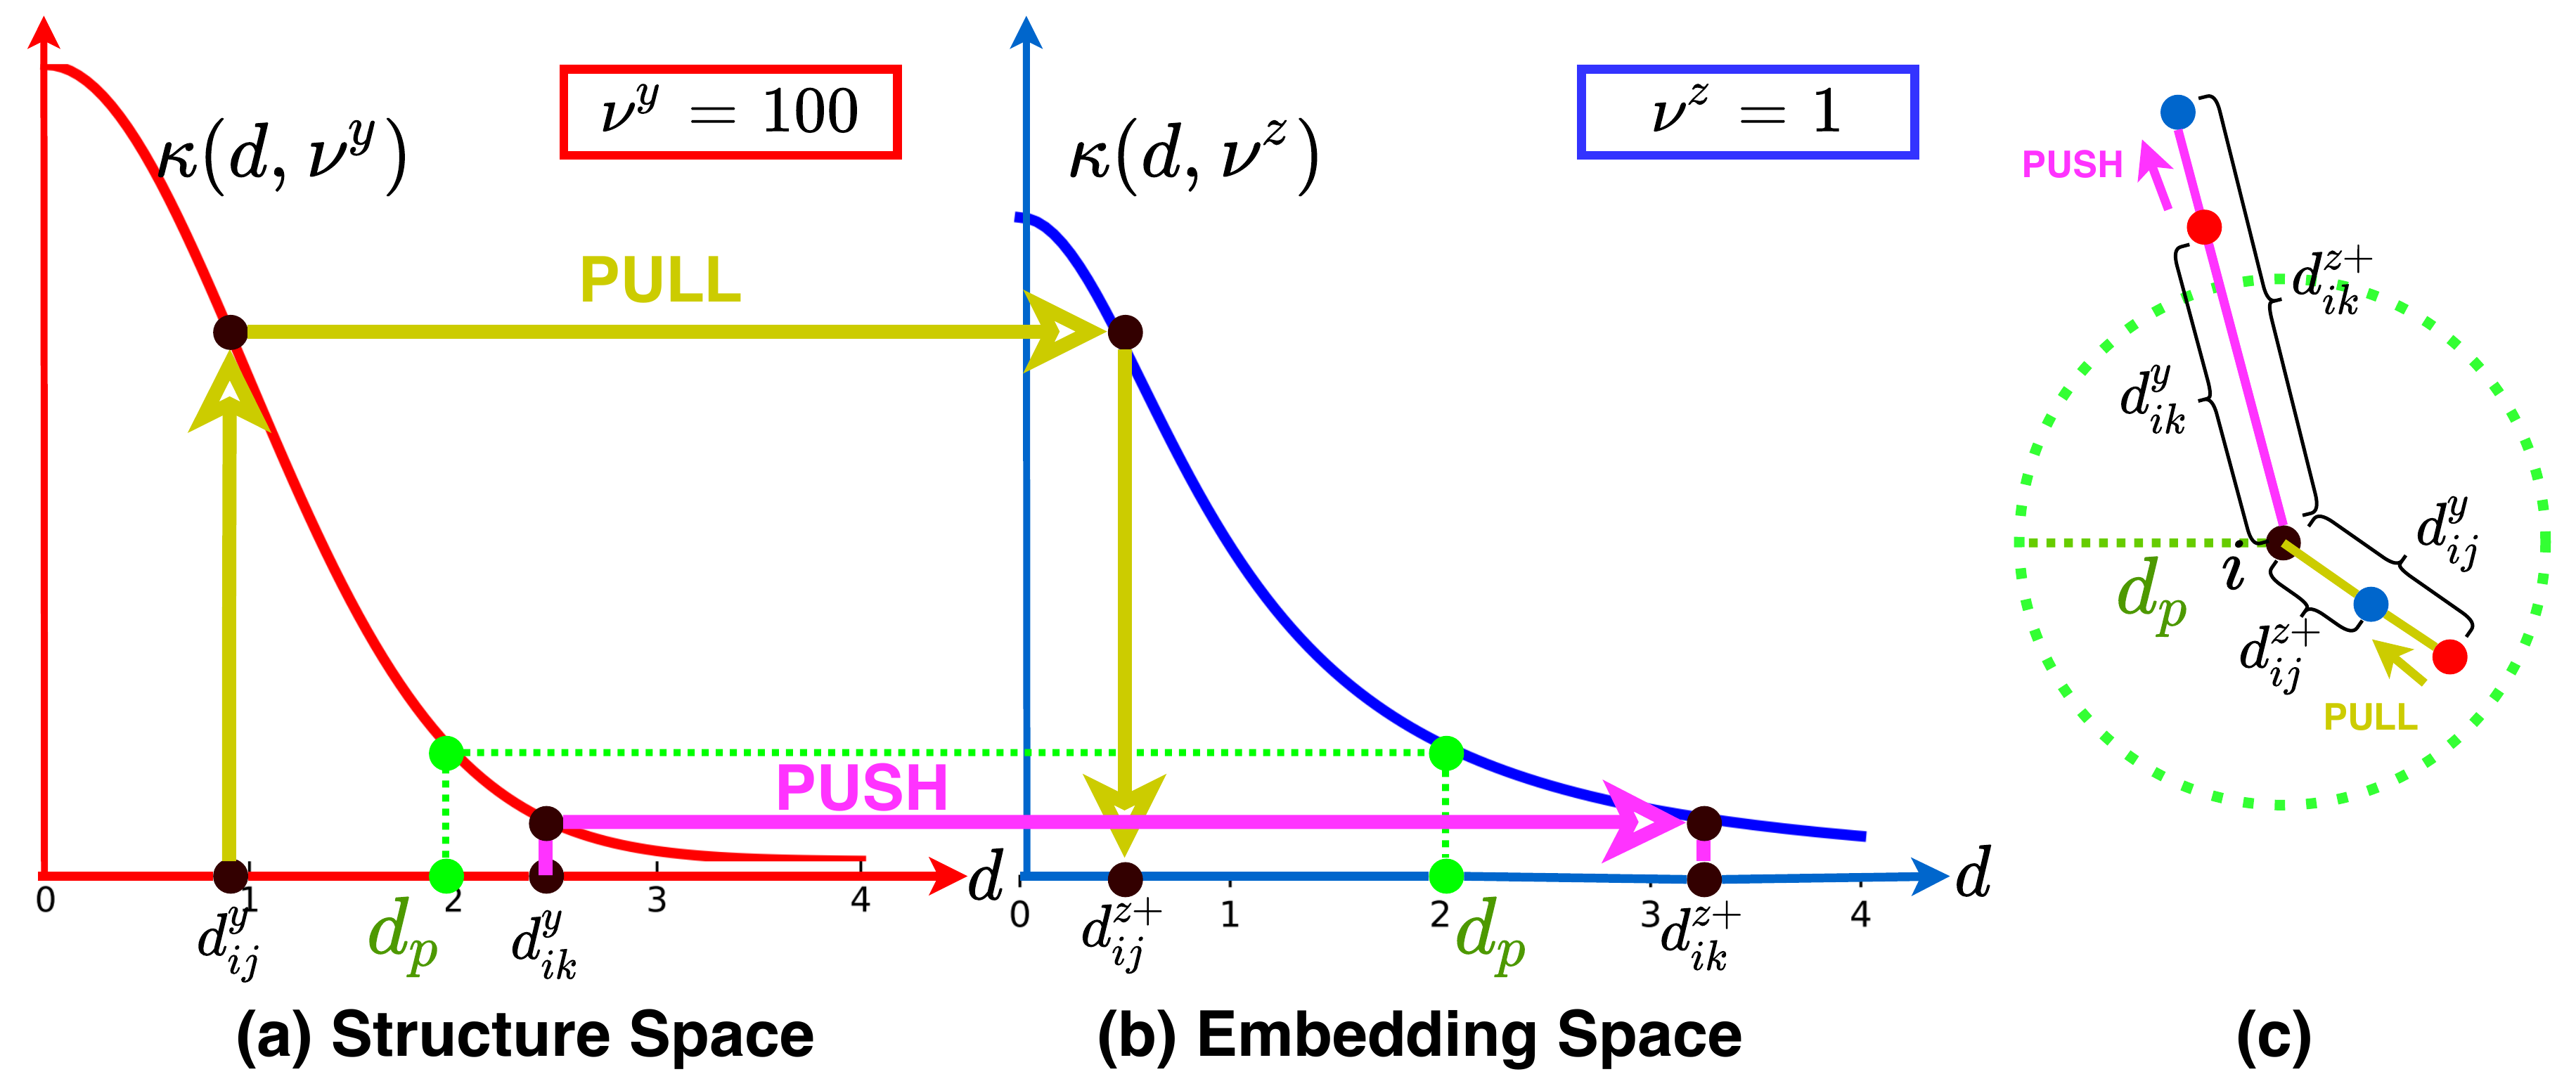}
  \caption{Proof. of Lemma 2}
  \label{fig:appendix_FIg-dl}
\end{figure}

\textbf{Proof.}

\begin{equation}
  \begin{aligned}
    L_{\text{D}} & \!= 
    \! E_{
      \substack{ 
          x_i, x_j   
          }    
      } 
      \left[
          \kappa \left(d^y ,\nu^y \right) 
          \log 
          \kappa \left( d^z_{ij} , \nu^z \right) 
          + 
          \left(1-\kappa \left(R_{ij}  d^y_{ij} ,\nu^y \right)\right)
          \log
          \left(1-\kappa \left( d^z_{ij} ,\nu^z \right)\right)
      \right]
    \\
  \end{aligned}
  \label{eq:appendix_dlme_}
\end{equation}

let $ d^y = R_{ij}  d^y_{ij}$ and let $d^z=d^z_{ij}$, we have,

\begin{equation}
  \begin{aligned}
    L_{\text{D}} & \!= 
    \! E_{
      \substack{ 
          x_i, x_j   
          }    
      } 
      \left[
          \kappa \left(d^y ,\nu^y \right) 
          \log 
          \kappa \left( d^z , \nu^z \right) 
          + 
          \left(1-\kappa \left(d^y ,\nu^y \right)\right)
          \log
          \left(1-\kappa \left( d^z ,\nu^z \right)\right)
      \right]
    \\
  \end{aligned}
  \label{eq:appendix_dlme__}
\end{equation}

then:

\begin{equation}
  \begin{aligned}
    \frac
      {\partial L_{\text{D}}}
      {\partial d^z}
    & \!= 
      E_{\substack{ x_i, x_j }} 
      \left[
          \kappa \left(d^y ,\nu^y \right)  
          \frac
            {1}
            {\kappa \left( d^z_{ij} , \nu^z \right)}
          \frac
            {\partial \kappa \left( d^z_{ij} , \nu^z \right)}
            {\partial d^z}
          + 
          \left(1-\kappa \left(d^y ,\nu^y \right)\right)
          \frac
            {-1}
            {1-\kappa \left(d^z_{ij} ,\nu^z \right)}
          \frac
            {\partial \kappa \left( d^z_{ij} , \nu^z \right)}
            {\partial d^z}
      \right]
    \\
    & \!= 
      E_{\substack{ x_i, x_j }} 
      \left[
        \frac
          {\partial \kappa \left( d^z_{ij} , \nu^z \right)}
          {\partial d^z}
        \left(
          \frac
            {\kappa \left(d^y ,\nu^y \right)  }
            {\kappa \left( d^z_{ij} , \nu^z \right)}
          -
          \frac
              {1-\kappa \left(d^y ,\nu^y \right)}
              {1-\kappa \left(d^z_{ij} ,\nu^z \right)}
        \right)
      \right]
    \\
    & \!= 
      E_{\substack{ x_i, x_j }} 
      \left[
        \frac
          {\partial \kappa \left( d^z_{ij} , \nu^z \right)}
          {\partial d^z}
        \left(
          \frac
            {
              \kappa \left(d^y ,\nu^y \right)
              \left(
                1-\kappa \left(d^z_{ij} ,\nu^z \right)
              \right)
              -
              \kappa \left( d^z_{ij} , \nu^z \right)
              \left(
                1-\kappa \left(d^y ,\nu^y \right)
              \right)
            }
            {
              \kappa \left( d^z_{ij} , \nu^z \right) 
              \left(
                1-\kappa \left(d^z_{ij} ,\nu^z \right)
              \right)
            }
        \right)
      \right]
    \\
    & \!= 
      E_{\substack{ x_i, x_j }} 
      \left[
        \frac
          {\partial \kappa \left( d^z_{ij} , \nu^z \right)}
          {\partial d^z}
        \left(
          \frac
            {
              \kappa \left(d^y ,\nu^y \right)
              -
              \kappa \left(d^y ,\nu^y \right)
              \kappa \left(d^z_{ij} ,\nu^z \right)
              -
              \kappa \left( d^z_{ij} , \nu^z \right)
              +
              \kappa \left( d^z_{ij} , \nu^z \right)
              \kappa \left(d^y ,\nu^y \right)
            }
            {
              \kappa \left( d^z_{ij} , \nu^z \right) 
              \left(
                1-\kappa \left(d^z_{ij} ,\nu^z \right)
              \right)
            }
        \right)
      \right]
    \\
    & \!= 
      E_{\substack{ x_i, x_j }} 
      \left[
        \frac
          {\partial \kappa \left( d^z_{ij} , \nu^z \right)}
          {\partial d^z}
        \left(
          \frac
            {
              \kappa \left(d^y ,\nu^y \right)
              -
              \kappa \left( d^z_{ij} , \nu^z \right)
            }
            {
              \kappa \left( d^z_{ij} , \nu^z \right) 
              \left(
                1-\kappa \left(d^z_{ij} ,\nu^z \right)
              \right)
            }
        \right)
      \right]
    \\
  \end{aligned}
  \label{eq:appendix_dlme___}
\end{equation}

Because $\kappa \left( d ,\nu^y \right) \in [0,1] $ is the kernel function of t-distribution. then they are Monotonically decreasing function in $d \in [0, +\infty]$
Then ${\partial L_{\text{D}}}/{\partial d^z}$ is the Monotonically decreasing function and when $\kappa \left(d^y ,\nu^y \right)-\kappa \left( d^z_{ij} , \nu^z \right) =0$ the ${\partial L_{\text{D}}}/{\partial d^z}=0$.

We take the optimal solution as:

\begin{equation}
    d^{z+} = \kappa^{-1}\left(\kappa(d^y, \nu^y), \nu^z\right)
\end{equation}
where $\kappa^{-1}(\cdot)$ is a inverse function of $\kappa(\cdot)$, and because $\kappa()$ is monotonically decreasing, the $\kappa^{-1}(\cdot)$ is monotonically decreasing.

Let $\Phi(d)= \kappa \left(d ,\nu^y \right)-\kappa \left( d , \nu^z \right) $, we have 

\begin{equation}
    \begin{aligned}
    \lim_{d \to +\infty} \Phi(d) &= \lim_{d \to +\infty} \kappa \left(d ,\nu^y \right)-\kappa \left( d , \nu^z \right)\\
    &= 
    % \lim_{d \to \infty} \kappa \left(d ,\nu^y \right)
    \lim_{d \to +\infty}
    \frac
        {\operatorname{Gam}\left(\frac{\nu^y +1}{2}\right)}
        {\sqrt{\nu^y  \pi} \operatorname{Gam}\left(\frac{\nu^y }{2}\right)}
    \left(
          1+\frac{d_{ij}^{2}}{\nu^y }
    \right)^{-\frac{\nu^y +1}{2}}
    -
    \lim_{d \to +\infty}
    \frac
        {\operatorname{Gam}\left(\frac{\nu^z +1}{2}\right)}
        {\sqrt{\nu^z  \pi} \operatorname{Gam}\left(\frac{\nu^z }{2}\right)}
    \left(
        1+\frac{d_{ij}^{2}}{\nu^z }
    \right)^{-\frac{\nu^z +1}{2}}\\
    &=0^{-}<0
    \end{aligned}
\end{equation}

and 

\begin{equation}
    \begin{aligned}
    \lim_{d \to 0^+} \Phi(d) &= \lim_{d \to +\infty} \kappa \left(d ,\nu^y \right)-\kappa \left( d , \nu^z \right)\\
    &= 
    % \lim_{d \to \infty} \kappa \left(d ,\nu^y \right)
    \lim_{d \to 0^+}
    \frac
        {\operatorname{Gam}\left(\frac{\nu^y +1}{2}\right)}
        {\sqrt{\nu^y  \pi} \operatorname{Gam}\left(\frac{\nu^y }{2}\right)}
    \left(
          1+\frac{d_{ij}^{2}}{\nu^y }
    \right)^{-\frac{\nu^y +1}{2}}
    -
    \lim_{d \to 0^+}
    \frac
        {\operatorname{Gam}\left(\frac{\nu^z +1}{2}\right)}
        {\sqrt{\nu^z  \pi} \operatorname{Gam}\left(\frac{\nu^z }{2}\right)}
    \left(
        1+\frac{d_{ij}^{2}}{\nu^z }
    \right)^{-\frac{\nu^z +1}{2}}\\
    &>0
    \\
    \end{aligned}
\end{equation}

And because the $\Phi(d)$ is a continuous function.

There must be $d_p$ let $\Phi(d)=0$, that is 

\begin{equation}
    \begin{aligned}
        \kappa \left(d_p ,\nu^y \right)-\kappa \left( d_p , \nu^z \right)=0 \\
        d_p = \kappa^{-1}\left(\kappa(d_p, \nu^y), \nu^z\right)
    \end{aligned}
\end{equation}

Then we solve for this particular point:

\begin{equation}
    \begin{aligned}
        \frac{\partial \Phi(d)}{\partial d^2} = 
            \frac
                {\operatorname{Gam}\left(\frac{\nu^y +1}{2}\right)}
                {\sqrt{\nu^y  \pi} \operatorname{Gam}\left(\frac{\nu^y }{2}\right)}
            ({-\frac{\nu^y +1}{2}})
            \left(
                  1+\frac{d_{ij}^{2}}{\nu^y }
            \right)^{-\frac{\nu^y +3}{2}}
            \frac{1}{v^y}
            -
            \frac
                {\operatorname{Gam}\left(\frac{\nu^z +1}{2}\right)}
                {\sqrt{\nu^z  \pi} \operatorname{Gam}\left(\frac{\nu^z }{2}\right)}
            ({-\frac{\nu^y +1}{2}})
            \left(
                1+\frac{d_{ij}^{2}}{\nu^z }
            \right)^{-\frac{\nu^z +3}{2}}
            \frac{1}{v^z} \\
        \frac{\partial \Phi(d)}{\partial d^2} = 
            \frac{1}{2\sqrt{\pi}}
            \left(
              \frac
              {\operatorname{Gam}\left(\frac{\nu^z +1}{2}\right)}
              {{\nu^z}^{1.5} \operatorname{Gam}\left(\frac{\nu^z }{2}\right)}
              (\nu^z +1)
              \left(
                1+\frac{d_{ij}^{2}}{\nu^z }
                \right)^{-\frac{\nu^z +3}{2}}
                % \frac{1}{v^z} 
                -
              \frac
                  {\operatorname{Gam}\left(\frac{\nu^y +1}{2}\right)}
                  {{\nu^y}^{1.5} \operatorname{Gam}\left(\frac{\nu^y }{2}\right)}
              (\nu^y +1)
              \left(
                    1+\frac{d_{ij}^{2}}{\nu^y }
              \right)^{-\frac{\nu^y +3}{2}}
              % \frac{1}{v^y}
            \right)
            \\
    \end{aligned}
\end{equation}

$\frac{\partial \Phi(d)}{\partial d^2}=0$ has a unique solution $d^*$, and $\frac{\partial \Phi(d^*)}{\partial d^2} < 0$.

\begin{figure}[h]
  \centering
  \includegraphics[width=2.2in]{fig/FIg-phi.pdf}
  \caption{Proof. of Lemma 2: $\Phi(d)$}
  \label{fig:appendix_FIg-dl2}
\end{figure}

Then $d_p$ is the only solution of $\Phi(d)=0$, and if $d>d_p$ then $\Phi(d)<0$, and if $d>d_p$ then $\Phi(d)<0$, and then $(d-d_p)\Phi(d)<0$.
Next we construct 
$\Psi (d)
= \kappa^{-1}(\kappa \left(d ,\nu^y \right), \nu^z)-\kappa^{-1} (\kappa \left( d , \nu^z \right), \nu^z) 
= \kappa^{-1}(\kappa \left(d ,\nu^y \right), \nu^z)-d$.

Because the $\kappa^{-1}(\cdot)$ is monotone continuity, if 
$$
\kappa \left(d ,\nu^y \right) > \kappa \left( d , \nu^z \right)
$$
then 
$$
\kappa^{-1}(\kappa \left(d ,\nu^y \right), \nu^z) < \kappa^{-1} (\kappa \left( d , \nu^z \right), \nu^z) = y
$$

Substitute $\Phi(d)= \kappa \left(d ,\nu^y \right)-\kappa \left( d , \nu^z \right)$ to $(d-d_p)\Psi(d)>0$, we have  $(d^y - d_p) (d^{z+} - d^y) >0$.
