# Supplementary material for: DLME: Deep Local-flatness Manifold Embedding
Source: arXiv:2207.03160 source file (2022-07-26)
Supplement: Supplementary file 3 [file Sec_appendix_proof_3.tex]

\clearpage

\subsection{A.3 Proof of Lemma 2}
\label{app_proof_3}

\ 
% \noindent \textbf{Lemma 3-1}. 
% Let two vectors $v_1=(i,j)$, $v_2=(j,k)$, where $i,j,k$ are three points, if we decreases the length of the vector $v_1$. the angle $ \alpha = \angle ijk$ will increase.

% \begin{figure}[t]
%   \centering
%   \includegraphics[width=6.2in]{figs/FIg-ijk.pdf}
%   \caption{Proof of Lemma 2}
%   \label{fig:appendix_lemma2}
% \end{figure}

\noindent\fbox{
  \parbox{0.99\textwidth}{
    \noindent \textbf{Lemma 2}. 
    Assume $f_\theta$ satisfies HOP1-2 order preserving:
    \begin{equation}
      \max ( \{ d_{ij}^y \}_{j \in \text{HOP}_1(x_i)} ) < \min ( \{ d_{ij}^y \}_{j \in \text{HOP}_2(x_i)})
    \end{equation}
    Then $\overline{K}_\mathcal{M}^{z+}<\overline{K}_\mathcal{M}^y$ where $\overline{K}_\mathcal{M}^y$ is the mean curvature in the structure space, and $\overline{K}_\mathcal{M}^{z+}$ is the mean curvature optimization results of $L_\text{D}$ in the embedding space.
    % Let $(i,j,k)$ be a discrete curve, where $x_j$ is the neighbor of the $x_i$, and $x_k$ is the non-neighbor of $x_i$. then, $C_{(i,j,k)}^e < C_{(i,j,k)}^s$, where $C_{(i,j,k)}^e$ and $C_{(i,j,k)}^s$ is the curvature of discrete curve $(i,j,k)$ in embedding and semantic space.
  }
}

\begin{figure}[t]
  \centering
  \includegraphics[width=4.2in]{fig/FIg-Page-14.pdf}
  \caption{Proof of Lemma 2}
  \label{fig:appendix_lemma2}
\end{figure}

We randomly select a point $j$ in the data set $X$, and then select 3 neighbor nodes $i,k_1,k_2$, while ensuring $k_1$ $k_2$ are the HOP2 of $i$.

As shown in Figure \ref{fig:appendix_lemma2},  Let $d_{ij}^y$, $d_{ik_1}^y$, $d_{ik_2}^y$ be distance in structure space,
and let $\angle 1=\angle jik_1$, $\angle 2=\angle jik_2$, $\angle 3=\angle k_1ik_2$. 
Because $j \in \text{HOP}_1(i)$ and $k_1, k_2 \in \text{HOP}_2(j)$, we have $d_{ik_1}^y>d_{ij}^y$ and $d_{ik_2}^y>d_{ij}^y$.

We can find a suitable $\alpha$ to make $d^y(ij)^y\alpha < d_p$ and $d^y(ik)^y\alpha > d_p$.
and let $d_1 = d_{ij}=\alpha d^y(ij)^y$,$d_2 = d_{ik_1}=\alpha d^y(ik_1)^y$,$d_3 = d_{ik_2}=\alpha d^y(ik_2)^y$.
Then according to Lemma 1, in the embedding sapce, $d^{z+}(ij)<d^y(ij)$ and $d(ik)^{z+}>d(ik)$ and.

First, according to Law of cosines\footnote{https://en.wikipedia.org/wiki/Law\_of\_cosines}, we have:

\begin{equation}
  \begin{aligned}
    d_{jk_1} = (d_1^2+d_2^2-2 d_1 d_2 \cos\angle1 )^\frac{1}{2}\\
    d_{jk_2} = (d_1^2+d_3^2-2 d_1 d_3 \cos\angle2 )^\frac{1}{2}\\
    d_{k_1k_2} = (d_2^2+d_3^2-2 d_2 d_3 \cos\angle3 )^\frac{1}{2}
    % d_{jk_1} = (d_1^2+d_2^2-2 d_1 d_2 \cos\angle1 )^\frac{1}{2}
  \end{aligned}
\end{equation}

According to discrete Gauss-Bonnet theorem, the discrete curvature of point $j$ is a function of $\angle ijk_1$, $\angle ijk_2$, $\angle k_1jk_2$. Let's write the three angle separately.

\begin{equation}
  \begin{aligned}
    \cos(\angle k_1jk_2)
    &= \frac{d_{jk_1}^2 + d_{jk_2}^2 -d_{k_1k_2}^2}{2d_{jk_1} d_{jk_2}}\\
    &= \frac
    {
      {(d_1^2+d_2^2-2 d_1 d_2 \cos\angle1 )^\frac{1}{2}}^2 
      +
      {(d_1^2+d_3^2-2 d_1 d_3 \cos\angle2 )^\frac{1}{2}}^2 
      -
      {(d_2^2+d_3^2-2 d_2 d_3 \cos\angle3 )^\frac{1}{2}}^2
    }{
      2
      {(d_1^2+d_2^2-2 d_1 d_2 \cos\angle1 )^\frac{1}{2}}
      {(d_1^2+d_3^2-2 d_1 d_3 \cos\angle2 )^\frac{1}{2}}
    }\\
    &= \frac
    {
      {(d_1^2+d_2^2-2 d_1 d_2 \cos\angle1 )}
      +
      {(d_1^2+d_3^2-2 d_1 d_3 \cos\angle2 )}
      -
      {(d_2^2+d_3^2-2 d_2 d_3 \cos\angle3 )}
    }{
      2
      {(d_1^2+d_2^2-2 d_1 d_2 \cos\angle1 )^\frac{1}{2}}
      {(d_1^2+d_3^2-2 d_1 d_3 \cos\angle2 )^\frac{1}{2}}
    }\\
    &= \frac
    {
      d_1^2
      -
      d_1d_2 \cos\angle1 
      -
      d_1d_3 \cos\angle2 
      +
      d_2d_3 \cos\angle3 
    }{
      {(d_1^2+d_2^2-2 d_1 d_2 \cos\angle1 )^\frac{1}{2}}
      {(d_1^2+d_3^2-2 d_1 d_3 \cos\angle2 )^\frac{1}{2}}
    }\\
    % d_{jk_1} = (d_1^2+d_2^2-2 d_1 d_2 \cos\angle1 )^\frac{1}{2}
  \end{aligned}
\end{equation}

% Let $d_1=1$, we have

% \begin{equation}
%   \begin{aligned}
%     \angle k_1jk_2 
%     &= \arccos(
%       \frac
%         {
%           d_2d_3 \cos\angle3 
%           -
%           d_2 \cos\angle1 
%           -
%           d_3 \cos\angle2 
%         }{
%           {(d_2^2-2  d_2 \cos\angle1 )^\frac{1}{2}}
%           {(d_3^2-2  d_3 \cos\angle2 )^\frac{1}{2}}
%         }
%     )\\
%     % d_{jk_1} = (d_1^2+d_2^2-2 d_1 d_2 \cos\angle1 )^\frac{1}{2}
%   \end{aligned}
% \end{equation}

% then we can calculate the $\angle ijk_1$, 

\begin{equation}
  \begin{aligned}
    \cos(\angle ijk_1) & = \frac{d_1^2 + d_{jk_1}^2 -d_2^2}{2d_1 d_{jk_1}} \\
    & = \frac{d_1^2 + {(d_1^2+d_2^2-2 d_1 d_2 \cos\angle1 )^\frac{1}{2}}^2 -d_2^2}{2d_1 {(d_1^2+d_2^2-2 d_1 d_2 \cos\angle1 )^\frac{1}{2}}} \\
    & = \frac{d_1^2 + d_1^2+d_2^2-2 d_1 d_2 \cos\angle1  -d_2^2}{2d_1 {(d_1^2+d_2^2-2 d_1 d_2 \cos\angle1 )^\frac{1}{2}}} \\
    & = \frac{d_1^2 - d_1d_2\cos\angle1}{d_1 {(d_1^2+d_2^2-2 d_1 d_2 \cos\angle1 )^\frac{1}{2}}} \\
    & = \frac{d_1 - d_2\cos\angle1}{{(d_1^2+d_2^2-2 d_1 d_2 \cos\angle1 )^\frac{1}{2}}}  \ \ \ \ \ \ \ \ \ \ \ \ \ \ \ \ \ \ \ \ \ \ \ \ \ \ \ \ \ \ \ \ \ \ \ \ \ \ \ \ \ \ \ \ \ \ \ \ \ \ \ \ \ \ \ \ \ \ \ \ \ \ \ \ \ \ \ \ \ \ \ \ \ \ \ \ \ \ \ \ \ \ \ \ \ \ \ \ \ \ \ \ \ \ \ \ 
    \\
    % d_{jk_1} = (d_1^2+d_2^2-2 d_1 d_2 \cos\angle1 )^\frac{1}{2}
  \end{aligned}
  \label{eq:angleijk1}
\end{equation}

% Let $d_1=1$, we have

% \begin{equation}
%   \begin{aligned}
%     \angle ijk_1 
%     & = \arccos (\frac{1 - d_2\cos\angle1}{{(1+d_2^2-2d_2 \cos\angle1 )^\frac{1}{2}}} )\\
%     % d_{jk_1} = (d_1^2+d_2^2-2 d_1 d_2 \cos\angle1 )^\frac{1}{2}
%   \end{aligned}
% \end{equation}

The same as Eq. (\ref{eq:angleijk1}):

\begin{equation}
  \begin{aligned}
    \cos(\angle ijk_2 )
    & = \frac{d_1 - d_3\cos\angle1}{{(d_1^2 + d_3^2 - 2d_1d_3 \cos\angle1 )^\frac{1}{2}}}
    % \arccos (\frac{1 - d_3\cos\angle2}{{(1+d_3^2-2d_3 \cos\angle2 )^\frac{1}{2}}} )
    \ \ \ \ \ \ \ \ \ \ \ \ \ \ \ \ \ \ \ \ \ \ \ \ \ \ \ \ \ \ \ \ \ \ \ \ \ \ \ \ \ \ \ \ \ \ \ \ \ \ \ \ \ \ \ \ \ \ \ \ \ \ \ \ \ \ \ \ \ \ \ \ \ \ \ \ \ \ \ \ \ \ \ \ \ \ \ \ \ \ \ \ \ 
    \\
    % d_{jk_1} = (d_1^2+d_2^2-2 d_1 d_2 \cos\angle1 )^\frac{1}{2}
  \end{aligned}
\end{equation}

Let $v_1 = \frac{d_2}{d_1}$, and $v_2 = \frac{d_3}{d_1}$, we directly represent three angles according to the inverse cosine function.

\begin{equation}
  \begin{aligned}
    \angle ijk_1 
    & = \arccos(\frac{1 - v_2\cos\angle1}{{(1 + v_2^2 - 2v_2 \cos\angle1 )^\frac{1}{2}}}) \\
    \angle ijk_2 
    & = \arccos(\frac{1 - v_3\cos\angle2}{{(1 + v_3^2 - 2v_3 \cos\angle2 )^\frac{1}{2}}}) \\
    \angle k_1jk_2 
    & = \arccos (
      \frac
        {
          1
          -
          v_1 \cos\angle1 
          -
          v_2 \cos\angle2 
          +
          v_1v_2 \cos\angle3 
        }{
          {(1 + v_1^2 - 2v_1 \cos\angle1 )^\frac{1}{2}}
          {(1 + v_2^2 - 2v_2 \cos\angle2 )^\frac{1}{2}}
        } 
    )
        \\
    % \arccos (\frac{1 - v_2\cos\angle2}{{(1+v_2^2-2v_2 \cos\angle2 )^\frac{1}{2}}} )
    % \ \ \ \ \ \ \ \ \ \ \ \ \ \ \ \ \ \ \ \ \ \ \ \ \ \ \ \ \ \ \ \ \ \ \ \ \ \ \ \ \ \ \ \ \ \ \ \ \ \ \ \ \ \ \ \ \ \ \ \ \ \ \ \ \ \ \ \ \ \ \ \ \ \ \ \ \ \ \ \ \ \ \ \ \ \ \ \ \ \ \ \ \ 
    \\
    % d_{jk_1} = (d_1^2+d_2^2-2 d_1 d_2 \cos\angle1 )^\frac{1}{2}
  \end{aligned}
\end{equation}

According to Lemma 1, $L_\text{D}$ will increase $d_2$ and $d_3$, and decreases $d_1$.
so  $L_\text{D}$ will increase $v_1$ amd $v_2$.

% \begin{equation}
%   \begin{aligned}
% % 
%   \end{aligned}
% \end{equation}

\begin{equation}
  \begin{aligned}
    & \frac{\partial \angle ijk_1}{\partial v_1} \\
    = 
    & \frac{\partial }{\partial v_1}
    \arccos (\frac{1 - v_1\cos\angle1}{{(1+v_1^2-2v_1 \cos\angle1 )^\frac{1}{2}}} ) \\
  =
  & \frac{-1}{1+\frac{(1 - v_1\cos\angle1)^2}{{(1+v_1^2-2v_1 \cos\angle1 )}}}
  \frac{\partial }{\partial v_1}
  \frac{1 - v_1\cos\angle1}{{(1+v_1^2-2v_1 \cos\angle1 )^\frac{1}{2}}} \\
  =
  & \frac
  {-(1+v_1^2-2v_1 \cos\angle1 )}
  {(1+v_1^2-2v_1 \cos\angle1 )+(1 - v_1\cos\angle1)^2}
  \frac{\partial }{\partial v_1}
  \frac{1 - v_1\cos\angle1}{{(1+v_1^2-2v_1 \cos\angle1 )^\frac{1}{2}}} \\
  =
  & \frac
  {-(1+v_1^2-2v_1 \cos\angle1 )}
  {(1+v_1^2-2v_1 \cos\angle1 )+(1 - v_1\cos\angle1)^2}
  % \frac{\partial }{\partial v_1}
  \left(
    \frac
    {
      -\cos\angle1({1+v_1^2-2v_1 \cos\angle1 )} 
      -
      (1 - v_1\cos\angle1)
      (v_1-\cos\angle1)
    }
    {(1+v_1^2-2v_1 \cos\angle1)^{\frac{3}{2}}}
  \right) \\
  =
  & 
  % \frac{\partial }{\partial v_1}
    \frac
    {
      (\cos\angle1)({1+v_1^2-2v_1 \cos\angle1 )} 
      +
      (1 - v_1\cos\angle1)
      (v_1-\cos\angle1)
    }
    {
      (1+v_1^2-2v_1 \cos\angle1)^{\frac{1}{2}}
      (1+v_1^2-2v_1 \cos\angle1 )+(1 - v_1\cos\angle1)^2
    }
  \\
  =
  & 
    \frac
    {
      v_1 - v_1\cos\angle1\cos\angle1
    }
    {
      (1+v_1^2-2v_1 \cos\angle1)^{\frac{1}{2}}
      \left((1+v_1^2-2v_1 \cos\angle1 )+(1 - v_1\cos\angle1)^2\right)
    }
    \\
    =
    & 
    \frac
    { \sin{\angle{1}}}
    {
      \left(
        v_{1}^{2} - 2 v_{1} \cos{\angle{1}} + 1
      \right)
    }
  \end{aligned}
  \label{eq:ijk1_d_v1}
\end{equation}

\begin{equation}
  \begin{aligned}
    &\frac{\partial \angle ijk_2}{\partial v_1} \\
    = 
    & \frac{\partial }{\partial v_1}
    \arccos (\frac{1 - v_2\cos\angle2}{{(1+v_2^2-2v_2 \cos\angle1 )^\frac{1}{2}}} ) 
    \ \ \ \ \ \ \ \ \ \ \ \ \ \ \ \ \ \ \ \ \ \ \ \ \ \ \ \ \ \ \ \ \ \
    \ \ \ \ \ \ \ \ \ \ \ \ \ \ \ \ \ \ \ \ \ \ \ \ \ \ \ \ \ \ \ \ \ \
    \ \ \ \ \ \ \ \ \ \ \ \ \ \ \ \ \ \ \ \ \ \ \ \ \ \ \ \ \ \ \ \ \ \ \ \ \ \ \ \ \ \ \ \ \ \ \ \ \ 
    \\
  = & 0
  \end{aligned}
  \label{eq:ijk2_d_v1}
\end{equation}

\begin{equation}
  \footnotesize
  \begin{aligned}
    & \frac{\partial \angle k_1jk_2}{\partial v_1} \\= 
    & \frac{\partial }{\partial v_1}
    \arccos (
      \frac
        {
          1
          -
          v_1 \cos\angle1 
          -
          v_2 \cos\angle2 
          +
          v_1v_2 \cos\angle3 
        }{
          {(1 + v_1^2 - 2v_1 \cos\angle1 )^\frac{1}{2}}
          {(1 + v_2^2 - 2v_2 \cos\angle2 )^\frac{1}{2}}
        } 
    )
  \\
  =
  &\frac{-1}{1+\frac{\left(v_1v_2 \cos\angle3 - v_1 \cos\angle1 - v_2\cos\angle2 \right)^2}{ {(v_1^2-2  v_1 cos\angle1 )} {(v_2^2-2  v_2 \cos\angle2 )}}}
    \frac{\partial }{\partial v_1}
    \frac{v_1v_2 \cos\angle3 - v_1 \cos\angle1 - v_2\cos\angle2 }{ {(v_1^2-2  v_1 cos\angle1 )^\frac{1}{2}} {(v_2^2-2  v_2 \cos\angle2 )^\frac{1}{2}}}
    \\
  % =
  % &\frac{-1}{1+\frac{\left(v_1v_2 \cos\angle3 - v_1 \cos\angle1 - v_2\cos\angle2 \right)^2}{ {(v_1^2-2  v_1 cos\angle1 )} {(v_2^2-2  v_2 \cos\angle2 )}}}
  %   \frac{\partial }{\partial v_1}
  %   \frac{v_1v_2 \cos\angle3 - v_1 \cos\angle1 - v_2\cos\angle2 }{ {(v_1^2-2  v_1 cos\angle1 )^\frac{1}{2}} {(v_2^2-2  v_2 \cos\angle2 )^\frac{1}{2}}}
  % \\
  =
  &\frac
  {-(v_1^2-2  v_1 cos\angle1 )(v_2^2-2  v_2 \cos\angle2 )}
  {(v_1^2-2  v_1 cos\angle1 )(v_2^2-2  v_2 \cos\angle2 )+\left(v_1v_2 \cos\angle3 - v_1 \cos\angle1 - v_2\cos\angle2 \right)^2}
  \frac{\partial }{\partial v_1}
  \frac{v_1v_2 \cos\angle3 - v_1 \cos\angle1 - v_2\cos\angle2 }{ {(v_1^2-2  v_1 cos\angle1 )^\frac{1}{2}} {(v_2^2-2  v_2 \cos\angle2 )^\frac{1}{2}}}
  \\
  =
  &\frac
  {-(v_1^2-2  v_1 cos\angle1 )(v_2^2-2  v_2 \cos\angle2 )}
  {(v_1^2-2  v_1 cos\angle1 )(v_2^2-2  v_2 \cos\angle2 )+\left(v_1v_2 \cos\angle3 - v_1 \cos\angle1 - v_2\cos\angle2 \right)^2}
  \frac{\partial }{\partial v_1}
  \frac{v_1v_2 \cos\angle3 - v_1 \cos\angle1 - v_2\cos\angle2 }{ {(v_1^2-2  v_1 cos\angle1 )^\frac{1}{2}} {(v_2^2-2  v_2 \cos\angle2 )^\frac{1}{2}}}
  \\
  % =&
  % \frac
  % {
  %   \frac{\left(2 v_1 - 2 \cos{\angle {1} }\right) \left(2 v_1 v_2 \cos{\left(\angle {3} \right)} - 2 v_1 \cos{\angle {1} } - 2 v_2 \cos{\left(\angle {2} \right)} + 2\right)}{4 \sqrt{\left(v_1^{2} - 2 v_1 \cos{\angle {1} } + 1\right) \left(v_2^{2} - 2 v_2 \cos{\left(\angle {2} \right)} + 1\right)} \left(v_1^{2} - 2 v_1 \cos{\angle {1} } + 1\right)} 
  %   -
  %   \frac{2 v_2 \cos{\left(\angle {3} \right)} - 2 \cos{\angle {1} }}{2 \sqrt{\left(v_1^{2} - 2 v_1 \cos{\angle {1} } + 1\right) \left(v_2^{2} - 2 v_2 \cos{\left(\angle {2} \right)} + 1\right)}}
  % }
  % {
  %   \sqrt{1 - \frac{\left(2 v_1 v_2 \cos{\left(\angle {3} \right)} - 2 v_1 \cos{\angle {1} } - 2 v_2 \cos{\left(\angle {2} \right)} + 2\right)^{2}}{4 \left(v_1^{2} - 2 v_1 \cos{\angle {1} } + 1\right) \left(v_2^{2} - 2 v_2 \cos{\left(\angle {2} \right)} + 1\right)}}
  % }
  % \\
  =&
  \frac
  {
    \left(
      v_1 v_2 \cos{\angle{1} } \cos{\angle{3} } 
      -
      v_1 v_2 \cos{\angle{2} } 
      + 
      v_1 \sin^{2}{\angle{1} } 
      +
      v_2 \cos{\angle{1} } \cos{\angle{2} } 
      -
      v_2 \cos{\angle{3} }
    \right)
  }
  {
    \sqrt{
      % \frac
      % {
        \left(v_1^{2} - 2 v_1 \cos{\angle{1} } + 1\right) 
        \left(v_2^{2} - 2 v_2 \cos{\angle{2} } + 1\right) 
        -
        \left(
          v_1 v_2 \cos{\angle{3} } 
          - 
          v_1 \cos{\angle{1} } 
          - 
          v_2 \cos{\angle{2} } 
          + 
          1
        \right)^{2}
      % }{
        % \left(v_1^{2} - 2 v_1 \cos{\angle{1} } + 1\right) 
        % \left(v_2^{2} - 2 v_2 \cos{\angle{2} } + 1\right)
      % }
    }
    \left(v_1^{2} - 2 v_1 \cos{\angle{1} } + 1\right)
    % \left(v_2^{2} - 2 v_2 \cos{\angle{2} } + 1\right)^{\frac{1}{2}}
  }
  \end{aligned}
  \label{eq:k1jk2_d_v1}
\end{equation}

% \begin{equation}
%   \begin{aligned}
%   & \frac{\partial }{\partial v_1}
%   \arccos (\frac{1 - v_2\cos\angle2}{{(1+v_2^2-2v_2 \cos\angle2 )^\frac{1}{2}}} ) = 0 
%   \\
%   \end{aligned}
% \end{equation}

Then, we sum Eq.(\ref{eq:ijk1_d_v1}) Eq.(\ref{eq:ijk2_d_v1}) Eq.(\ref{eq:k1jk2_d_v1}) together.

\begin{equation}
  % \footnotesize
  \begin{aligned}
    &\frac{\partial \angle ijk_1 + \angle ijk_2 + \angle k_1jk_2}{\partial v_1} \\
    =&  
    \frac{\partial }{\partial v_1}[
    \arccos (\frac{1 - v_2\cos\angle2}{{(1+v_2^2-2v_2 \cos\angle2 )^\frac{1}{2}}} ) 
    +
    \arccos (\frac{1 - v_1\cos\angle1}{{(1+v_1^2-2v_1 \cos\angle1 )^\frac{1}{2}}} )
    +
    \frac{1 - v_1\cos\angle1}{{(1 + v_1^2 - 2v_1\cos\angle1 )^\frac{1}{2}}} ]\\
    =&
    \frac
    {
      \left(
        v_1 v_2 \cos{\angle{1} } \cos{\angle{3} } 
        -
        v_1 v_2 \cos{\angle{2} } 
        + 
        v_1 \sin^{2}{\angle{1} } 
        +
        v_2 \cos{\angle{1} } \cos{\angle{2} } 
        -
        v_2 \cos{\angle{3} }
      \right)
    }
    {
      \sqrt{
        % \frac
        % {
          \left(v_1^{2} - 2 v_1 \cos{\angle{1} } + 1\right) 
          \left(v_2^{2} - 2 v_2 \cos{\angle{2} } + 1\right) 
          -
          \left(
            v_1 v_2 \cos{\angle{3} } 
            - 
            v_1 \cos{\angle{1} } 
            - 
            v_2 \cos{\angle{2} } 
            + 
            1
          \right)^{2}
        % }{
          % \left(v_1^{2} - 2 v_1 \cos{\angle{1} } + 1\right) 
          % \left(v_2^{2} - 2 v_2 \cos{\angle{2} } + 1\right)
        % }
      }
      \left(v_1^{2} - 2 v_1 \cos{\angle{1} } + 1\right)
      % \left(v_2^{2} - 2 v_2 \cos{\angle{2} } + 1\right)^{\frac{1}{2}}
    }\\
    &+
    \frac
    { \sin{\angle{1}}}
    {
      % \sqrt{
        % \frac
        % {\sin{\angle{1}}}
        % {v_1^{2} - 2 v_1 \cos{\angle{1}} + 1}
      % }
      \left(
        v_1^{2} - 2 v_1 \cos{\angle{1}} + 1
      \right)
    }+0\\
    =&
    \frac
    {
      \left(
        v_1 v_2 \cos{\angle{1} } \cos{\angle{3} } 
        -
        v_1 v_2 \cos{\angle{2} } 
        + 
        v_1 \sin^{2}{\angle{1} } 
        +
        v_2 \cos{\angle{1} } \cos{\angle{2} } 
        -
        v_2 \cos{\angle{3} }
      \right)
      +
      \sin{\angle{1}}
      M_1
    }
    {
      M_1
      \left(v_1^{2} - 2 v_1 \cos{\angle{1} } + 1\right)
      % \left(v_2^{2} - 2 v_2 \cos{\angle{2} } + 1\right)^{\frac{1}{2}}
    }
    \\
  \end{aligned}
\end{equation}

where $M_1=\sqrt{
  % \frac
  % {
    \left(v_1^{2} - 2 v_1 \cos{\angle{1} } + 1\right) 
    \left(v_2^{2} - 2 v_2 \cos{\angle{2} } + 1\right) 
    -
    \left(
      v_1 v_2 \cos{\angle{3} } 
      - 
      v_1 \cos{\angle{1} } 
      - 
      v_2 \cos{\angle{2} } 
      + 
      1
    \right)^{2}
  % }{
    % \left(v_1^{2} - 2 v_1 \cos{\angle{1} } + 1\right) 
    % \left(v_2^{2} - 2 v_2 \cos{\angle{2} } + 1\right)
  % }
}$

Let $\phi=      \left(
  v_1 v_2 \cos{\angle{1} } \cos{\angle{3} } 
  -
  v_1 v_2 \cos{\angle{2} } 
  + 
  v_1 \sin^{2}{\angle{1} } 
  +
  v_2 \cos{\angle{1} } \cos{\angle{2} } 
  -
  v_2 \cos{\angle{3} }
\right)
+
\sin{\angle{1}}
M_1$

\begin{equation}
  \begin{aligned}
    & \frac{\partial \phi}{\partial v_1}
    =\left(
      v_2 \cos{\angle{1} } \cos{\angle{3} } 
      -
      v_2 \cos{\angle{2} } 
      + 
      \sin^{2}{\angle{1} } 
    \right)
    +
    \sin{\angle{1}}
    \frac{\partial M_1}{\partial v_1}\\
    % \frac{\left(v_{2} - \cos{\left(a_{1} \right)}\right) \left(v_{3}^{2} - 2 v_{3} \cos{\left(a_{2} \right)} + 1\right) - \left(v_{3} \cos{\left(a_{3} \right)} - \cos{\left(a_{1} \right)}\right) \left(v_{2} v_{3} \cos{\left(a_{3} \right)} - v_{2} \cos{\left(a_{1} \right)} - v_{3} \cos{\left(a_{2} \right)} + 1\right)}{\sqrt{\left(v_{2}^{2} - 2 v_{2} \cos{\left(a_{1} \right)} + 1\right) \left(v_{3}^{2} - 2 v_{3} \cos{\left(a_{2} \right)} + 1\right) - \left(v_{2} v_{3} \cos{\left(a_{3} \right)} - v_{2} \cos{\left(a_{1} \right)} - v_{3} \cos{\left(a_{2} \right)} + 1\right)^{2}}}
  \end{aligned}
\end{equation}

\begin{equation}
  \begin{aligned}
    \frac{\partial M_1}{\partial v_1}
    & =
    \frac{\left(v_{2} - \cos{\left(a_{1} \right)}\right) \left(v_{3}^{2} - 2 v_{3} \cos{\left(a_{2} \right)} + 1\right) - \left(v_{3} \cos{\left(a_{3} \right)} - \cos{\left(a_{1} \right)}\right) \left(v_{2} v_{3} \cos{\left(a_{3} \right)} - v_{2} \cos{\left(a_{1} \right)} - v_{3} \cos{\left(a_{2} \right)} + 1\right)}{\sqrt{\left(v_{2}^{2} - 2 v_{2} \cos{\left(a_{1} \right)} + 1\right) \left(v_{3}^{2} - 2 v_{3} \cos{\left(a_{2} \right)} + 1\right) - \left(v_{2} v_{3} \cos{\left(a_{3} \right)} - v_{2} \cos{\left(a_{1} \right)} - v_{3} \cos{\left(a_{2} \right)} + 1\right)^{2}}}
  \end{aligned}
\end{equation}

Let $M_2={\left(v_{2} - \cos{\left(a_{1} \right)}\right) \left(v_{3}^{2} - 2 v_{3} \cos{\left(a_{2} \right)} + 1\right) - \left(v_{3} \cos{\left(a_{3} \right)} - \cos{\left(a_{1} \right)}\right) \left(v_{2} v_{3} \cos{\left(a_{3} \right)} - v_{2} \cos{\left(a_{1} \right)} - v_{3} \cos{\left(a_{2} \right)} + 1\right)}$

\begin{equation}
  \begin{aligned}
    \frac{\partial M2}{\partial v_1}
    & =
    v_2^{2} - 2 v_2 \cos{\left(\angle {2} \right)} + \left(- v_2 \cos{\left(\angle {3} \right)} + \cos{\angle {1} }\right) \left(v_2 \cos{\left(\angle {3} \right)} - \cos{\angle {1} }\right) + 1\\
    & =
    v_2^{2} - 2 v_2 \cos{\left(\angle {2} \right)} + \left(- v_2 \cos{\left(\angle {3} \right)} + \cos{\angle {1} }\right) \left(v_2 \cos{\left(\angle {3} \right)} - \cos{\angle {1} }\right) + 1\\
    % & =
    % - v_2^{2} \cos^{2}{\left(\angle {3} \right)} + v_2^{2} + 2 v_2 \cos{\angle {1} } \cos{\left(\angle {3} \right)} - 2 v_2 \cos{\left(\angle {2} \right)} - \cos^{2}{\angle {1} } + 1\\
    & =
    v_2^{2} \sin^{2}{\left(\angle {3} \right)} 
    + 2 v_2 
    \left(
      \cos{\angle {1} } \cos{\left(\angle {3} \right)} - \cos{\left(\angle {2} \right)} 
    \right)
    +
    \sin^{2}{\angle {1} } \\
    % & =
    % v_2^{2} \sin^{2}{\left(\angle {3} \right)} 
    % - 2 v_2 
    % \left(
    %   \sin{\angle {1} } \sin{\left(\angle {3} \right)} \cos{\left(\angle P \right)} 
    % \right)
    % +
    % \sin^{2}{\angle {1} } \\
    & >
    v_2^{2} \sin^{2}{\left(\angle {3} \right)} 
    - 2 v_2 
    \left(
      \sin{\angle {1} } \sin{\left(\angle {3} \right)}
    \right)
    +
    \sin^{2}{\angle {1} } \\
    & >
    \left(
      v_2^{2} \sin{\left(\angle {3} \right)} 
      -
      \sin{\angle {1} } 
    \right)^2 > 0
    \\
  \end{aligned}
\end{equation}

So

\begin{equation}
  \begin{aligned}
    M_1 
    &> 
    v_2^{2} - 2 v_2 \cos{\left(\angle{2} \right)} - \left(- v_2 \cos{\left(\angle{2} \right)} + 1\right)^{2} + 1 \\
    &> 
    - v_{3}^{2} \cos^{2}{\left(\angle_{2} \right)} + v_{3}^{2} \\
    &> 
    v_{3}^{2} \sin^{2}{\left(\angle_{2} \right)} \\
    &> 
    0
  \end{aligned}
\end{equation}

So $\frac{\partial M2}{\partial v_1}> \frac{\partial M2}{\partial v_1} |_{d2=1} = v_2 \sin\angle 3 -v_2\sin \angle 1$, So 

So
\begin{equation}
  \begin{aligned}
    & \frac{\partial \phi}{\partial v_1}
    =\left(
      v_2 \cos{\angle{1} } \cos{\angle{3} } 
      -
      v_2 \cos{\angle{2} } 
      + 
      \sin^{2}{\angle{1} } 
    \right)
    +
    \sin{\angle{1}}
    \frac{\partial M_1}{\partial v_1}\\
    &>
    v_2
    \left(
       \cos{\angle{1} } \cos{\angle{3} } 
      -
      \cos{\angle{2} } 
    \right)
    + 
      \sin^{2}{\angle{1} } 
    +
    \sin{\angle{1}}
    {\frac{\partial M_1}{\partial v_1}}_{d2=1}\\
    &>
    v_2
    \left(
      \sin{\angle{1} } \sin{\angle{3} } \cos P
      + 
      \sin^{2}{\angle{1} } 
    \right)
    +
    \sin{\angle{1}}
    (v_2 \sin\angle 3 -v_2\sin \angle 1)\\
    &>
    \sin{\angle{1} }
    \left( 
      v_2
      \left(
        -1\sin{\angle{3} } \cos P
        + 
        \sin{\angle{1} } 
        \right)
        +
       v_2 \sin\angle 3 -v_2\sin \angle 1
    \right) \\
    &> 0\\
      \end{aligned}
\end{equation}

So $\frac{\partial \angle A}{\partial v_1}>0$, and 
because $v_1^{z+}>v_1^{y}$ so $K_j^{z+} = K_j^{y} - \int_{v_1^{y}}^{v_1^{z+}} \frac{\partial \angle A}{\partial v_1} \,d v_1 $, and $K_j^{z+}<K_j^{y}$.
