# Supplementary material for: DLME: Deep Local-flatness Manifold Embedding
Source: arXiv:2207.03160 source file (2022-07-26)
Supplement: Supplementary file 4 [file Sec_appendix_relatedworks.tex]

The manifold learning consists of two sub-processes: \emph{structure modeling} and \emph{low-dimensional embedding}.
(1) relationships modeling quantifies the relationships (similarity or dissimilarity) of the input data by linear or nonlinear methods, and (2) low-dimensional embedding refers to the representation of the relationships obtained by `structure modeling' into a low-dimensional space.
% All manifold learning methods can be seen as proposing innovations in at least one of these two sub-steps.
All other manifold learning methods are summarized into these two sub-processes.

We divide all methods into four categories according to whether \textbf{uses neural networks} and whether \textbf{uses similarity}.

The first category (C1) is that the method neither uses neural networks nor is based on similarity (shown in table \ref{tab:relatedwork}).
In the \textbf{baseline approach}, MDS \cite{kruskal1964nonmetric} relies on distance ("dissimilarity") to model relationships linearly and characterize them linearly in low-dimensional space.
ISOMAP \cite{tenenbaum_global_2000} improves the description of high-dimensional manifolds by using geodesic distances instead of linear modeling based on MDS.
Similarly, LLE \cite{roweis_nonlinear_2000} introduces the assumption of linearity for localized manifolds, improving the MDS to model linearly only locally.
Laplacian Eigenmap (LapEig) \cite{liu2018spectral} introduces undirected graphs in the modeling process and improves the representation process using graph embedding methods.

The second category (C2) is that methods do not use neural networks but are based on similarity.
Some methods model the input space data carefully by introducing distribution priors to design additional optimization tasks.
The SNE \cite{hinton_stochastic_2003} method assumes that the data metrics in both the input space and the latent space satisfy the normal distribution, determines the appropriate Normal distribution parameter $\sigma$ by relying on dichotomous search, and then uses the normal distribution as the kernel function to transform the distance into similarity for modeling. And the representation process is completed with the optimization goal of the best match between latent space similarity and data space similarity.
Based on SNE, t-SNE \cite{maaten_visualizing_2008}, and LargeVis\cite{Tang2016largevis} replaces the kernel function of latent space with the standard long-tailed t-distribution, thus achieving a better visualization effect.
UMAP \cite{mcinnes_umap_2018} introduces the assumption of locally uniform manifolds based on extensive theoretical analysis and makes a significant improvement in computational cost.

The third category (C3) is methods that use neural networks but are not based on similarity.
These methods have abandoned nonlinear complex modeling schemes and instead use direct metrics on the data space to build an end-to-end model.
For example, Topological autoencoder (TAE) \cite{moor2020topological} and Geometry Regularized AutoEncoders (GRAE) \cite{duque2020extendable} train autoencoders directly with constraints on the local distance in the input space.
IVIS \cite{szubert_structure_preserving_2019} Train the neural network by designing triplet loss function with distance as a constraint.
Due to insufficient modeling, this type of approach is often used in smaller nonlinear biological domains and cannot handle complex image and semantic data. There are no deep manifold learning methods that accurately model the input manifold with the help of networks.

The last category (C4) of methods uses neural networks and is based on similarity.
Meanwhile, some scholars have proposed some deep popular learning schemes by combining deep learning with manifold learning.
Parametric t-SNE (P-TSNE) \cite{maaten_learning_2009} and Parametric UMAP (P-UMAP) \cite{sainburg_parametric_2021} replace the modeling part with neural networks on top of t-SNE and UMAP, giving the methods the ability to process unseen data. Both ways still follow the same pattern of relationship modeling via dichotomous lookup, so they are not strictly speaking end-to-end scenarios.

\begin{table}[h]
    \caption{Important state-of-the-art manifold learning methods}
    \small
    \centering
    \begin{tabular}{c|c|cc|cc}
        \toprule
        \multicolumn{2}{l|}{\multirow{2}{*}{}} & \multicolumn{2}{c|}{Two Sub-processes of Manifold Learning}               & \multicolumn{2}{c}{Embedding Ability}                                                                                                                                                                                                                                                                                  \\ \cline{3-6}
        \multicolumn{2}{l|}{}                  & \begin{tabular}[c]{@{}c@{}}How to \\ `Structure\\Modeling'\end{tabular}   & \begin{tabular}[c]{@{}c@{}}How to \\`Low-dimensional\\Embedding'\end{tabular} & \begin{tabular}[c]{@{}c@{}}Simple\\Manifold\\{\scriptsize(Tabular Data)}\end{tabular} & \begin{tabular}[c]{@{}c@{}}Complex\\Manifold\\{\scriptsize (Image Data)}\end{tabular}              \\ \midrule
        \multirow{4}{*}{C1}                    & MDS                                                                       & Euclidean Distance                                                            & Euclidean Distance                                                                                          & \checkmark                                                                                                  & $\times$   \\
                                               & ISOMAP                                                                    & Geodesic Distance                                                             & Euclidean Distance                                                                                          & \checkmark                                                                                                  & $\times$   \\
                                               & LLE                                                                       & Local Euclidean Distance                                                      & Euclidean Distance                                                                                          & \checkmark                                                                                                  & $\times$   \\
                                               & LapEig                                                                    & Nearest Neighbor Graph                                                        & Spectral Embedding                                                                                          & \checkmark                                                                                                  & $\times$   \\ \midrule
        \multirow{3}{*}{C2}                    & SNE                                                                       & Gaussian Kernel                                                               & Gaussian Kernel                                                                                             & \checkmark                                                                                                  & $\times$   \\
                                               & t-SNE                                                                     & Gaussian Kernel                                                               & t-Kernel                                                                                                    & \checkmark                                                                                                  & $\times$   \\
                                               & UMAP                                                                      & Gaussian Kernel                                                               & Custom Kernel                                                                                               & \checkmark                                                                                                  & $\times$   \\ \midrule
        \multirow{3}{*}{C3}                    & TAE                                                                       & Local Euclidean Distance                                                      & NN + PH Loss                                                                                                & \checkmark                                                                                                  & $\times$   \\
                                               & GRAE                                                                      & Local Euclidean Distance                                                      & NN + Distance Loss                                                                                          & \checkmark                                                                                                  & $\times$   \\
                                               & IVIS                                                                      & Local Euclidean Distance                                                      & NN + triplet loss                                                                                           & \checkmark                                                                                                  & $\times$   \\ \midrule
        \multirow{3}{*}{C4}                    & P-TSNE                                                                    & Gaussian Kernel                                                               & NN + t-Kernel                                                                                               & \checkmark                                                                                                  & $\times$   \\
                                               & P-UMAP                                                                    & Gaussian Kernel                                                               & NN + Custom Kernel                                                                                          & \checkmark                                                                                                  & $\times$   \\
                                               & \begin{tabular}[c]{@{}c@{}}\textbf{Our} \\ \textbf{Proposed}\end{tabular} & NN + Priori Knowledge                                                         & NN + t-kernel                                                                                               & \checkmark                                                                                                  & \checkmark \\
        \bottomrule
    \end{tabular}
    \label{tab:relatedwork}
\end{table}

% \clearpage
