# Supplementary material for: DLME: Deep Local-flatness Manifold Embedding
Source: arXiv:2207.03160 source file (2022-07-26)
Supplement: Supplementary file 5 [file Sec_appendix_setting_complex.tex]

\subsection{Experimental setups:}

% The compared methods include 
The compared methods include contrastive learning methods (
    NPID \cite{wu_unsupervised_2018} \footnote{https://github.com/zhirongw/lemniscate.pytorch} , 
    ODC \cite{zhan2020online} \footnote{https://github.com/open-mmlab/OpenSelfSup}, 
    SimCLR \cite{chen_simple_2020} \footnote{https://github.com/google-research/simclr}, 
    MOCO.v2 \cite{he_momentum_2020} \footnote{https://github.com/facebookresearch/moco} and 
    BYOL \cite{grill_bootstrap_2020} \footnote{https://github.com/deepmind/deepmind-research/tree/master/byol} 
)
and contrastive clustering methods (
    DAC \cite{haeusser_associative_2019} \footnote{https://github.com/jplapp/associative\_deep\_clustering}, 
    % DDC \cite{chang_deep_2019}, 
    DCCM \cite{wu_deep_2019-1} \footnote{https://github.com/Cory-M/DCCM}, 
    % IIC \cite{ji_invariant_2019} \footnote{https://github.com/xu-ji/IIC}, 
    PICA \cite{huang_deep_2020} \footnote{https://github.com/Raymond-sci/PICA} 
    CC \cite{li_contrastive_2020} \footnote{https://github.com/Yunfan-Li/Contrastive-Clustering}, and 
    CRLC \cite{do2021clustering}    
).
The datasets include four image datasets (
  CIFAR10\footnote{https://www.cs.toronto.edu/~kriz/cifar.html},
  CIFAR100\footnote{https://www.cs.toronto.edu/~kriz/cifar.html},
  STL10\footnote{https://cs.stanford.edu/~acoates/stl10/}, and
  tinyImageNet \footnote{https://www.kaggle.com/c/tiny-imagenet}
)

To compare with the two different baseline methods, the segmentation of the dataset used by the two subtasks is various.

\begin{table*}[h]   
  \centering
  \caption{Dataset segmentation of linear-test sub-task}
  \begin{tabular}{cccccc}
    \hline \text { Dataset }    & \text { Train data }        & \text { Test data }  & \text { Train Samples } & \text { Test Samples } & \text { Classes } \\
    \hline \text { CIFAR-10 }   & \text { Train }             & \text { Test }       & 50,000                  & 10,000                 & 10 \\
    \text { CIFAR-100 }         & \text { Train }             & \text { Test }       & 50,000                  & 10,000                 & 100 \\
    \text { STL-10 }            & \text { Train + Unlabeled}  & \text { Test }       & 5,000+100,000           & 8,000                  & 10 \\
    \text { Tiny-ImageNet }     & \text { Train }             & \text { Test }       & 100,000                 & 100,000                & 200 \\
    \hline
  \end{tabular}
  \label{at:6}
\end{table*}

\begin{table*}[h]
  \centering
  \caption{Dataset segmentation of clustering sub-task}
  \begin{tabular}{cccc}
      \hline \text { Dataset }    & \text { Split }       & \text { Samples } & \text { Classes } \\
      \hline \text { CIFAR-10 }   & \text { Train+Test }  & 60,000            & 10 \\
      \text { CIFAR-100 }         & \text { Train+Test }  & 60,000            & 20 \\
      \text { STL-10 }            & \text { Train+Test }  & 13,000            & 10 \\
      \text { Tiny-ImageNet }     & \text { Train }       & 100,000           & 200 \\
      \hline
  \end{tabular}
  \label{at:8}
\end{table*}

\subsection{Experimental parameters for linear-test sub-task}

For fire compared with BYOL \cite{grill_bootstrap_2020} and other methods, we use the same ResNet-50 architecture as the $f_\theta$ and use MLP as $g_\phi$.
The performance of two downstream tasks is evaluated in the embedding space.
we use the Adamw optimizer and weight decay is 1e-6. 
$\nu_y=100$, $\nu_z=10$,
We use the same data augmentation method as BYOL \cite{grill_bootstrap_2020}.

We use the grid search method to determine the best super parameters. The super parameters adjusted in the grid search method are as follows.

\begin{table}[!htbp]
  \begin{center}
    \caption{Hyperparameter search space for linear-test sub-task}
    % \label{tab:A2}
    \begin{tabular}{lc}
    \hline
    Hyperparameters & Search Space \\ \hline
    % Data augmentation KNN $K$ & {[}5, 10, 15, 20{]} \\ \hline
    % degree of freedom in embedding space $\nu^z$ & {[}0.1, 0.01{]} \\ \hline
    batch size        & {[}256, 512{]} \\ \hline
    learning rate     & {[}2e-4, 5e-4, 6e-4{]} \\ \hline
    \end{tabular}
  \end{center}
\end{table}

\subsection{Experimental parameters for clustering sub-task}

For fire compared with CC \cite{li_contrastive_2020} and other methods, we use the same ResNet-50 architecture as the $f_\theta$ and use MLP as $g_\phi$.
The performance of two downstream tasks is evaluated in the embedding space.
we use the AdamW optimizer and weight decay is 1e-6. 
$\nu_y=100$,
We use the same data augmentation method as BYOL \cite{grill_bootstrap_2020}.

\begin{table}[!htbp]
  \begin{center}
    \caption{Hyperparameter search space for clustering sub-task}
    % \label{tab:A2}
    \begin{tabular}{lc}
    \hline
    Hyperparameters & Search Space \\ \hline
    % Data augmentation KNN $K$ & {[}5, 10, 15, 20{]} \\ \hline
    degree of freedom in embedding space $\nu^z$ & {[}1, 100, 100{]} \\ \hline
    batch size        & {[}128, 256, 512{]} \\ \hline
    learning rate     & {[}1e-4, 2e-4, 1e-3{]} \\ \hline
    \end{tabular}
  \end{center}
\end{table}
