# Supplementary material for: DLME: Deep Local-flatness Manifold Embedding
Source: arXiv:2207.03160 source file (2022-07-26)
Supplement: Supplementary file 7 [file Sec_appendix.tex]

% \newtheorem{innercustomlemma}{Lemma}


% \section{Experiments Details}

% \section{Experiments Details in Easy Datasets}

% \subsection{More detailed experiments}

% To test the stability of DLME, we counted the performance of 5 different seeds as shown in Table \ref{tab_seed5}.

% \begin{table*}[h]
%     \centering
%     \small
%     \caption{5 different seeds' Performance of on }
%     \begin{tabular}{@{}ccc|ccc@{}}
%         \toprule
%         \multicolumn{3}{c|}{STL-10}            & \multicolumn{3}{c}{Tiny-ImageNet}    \\ \midrule
%         Seed    & ACC1         & ACC5         & Seed    & ACC1         & ACC5         \\ \midrule
%         0       & 90.013       & 99.588       & 0       & 44.8         & 70.74        \\
%         1       & 89.138       & 99.613       & 1       & 44.94        & 70.96        \\
%         2       & 89.363       & 99.6         & 2       & 44.58        & 71.06        \\
%         3       & 89.538       & 99.5         & 3       & 44.72        & 71.36        \\
%         4       & 89.675       & 99.625       & 4       & 44.2         & 71.58        \\
%         Average & 89.54(0.32)  & 99.58(0.049) & Average & 44.648(0.28) & 71.14(0.33)  \\ \midrule
%         \multicolumn{3}{c|}{Cifar-100}         & \multicolumn{3}{c}{Cifar-10}         \\ \midrule
%         Seed    & ACC1         & ACC5         & Seed    & ACC1         & ACC5         \\ \midrule
%         0       & 64.99        & 89.29        & 0       & 91.23        & 99.81        \\
%         1       & 66.07        & 89.83        & 1       & 91.08        & 99.81        \\
%         2       & 65.12        & 89.21        & 2       & 91.26        & 99.8         \\
%         3       & 66.1         & 90.04        & 3       & 91.19        & 99.82        \\
%         4       & 65.65        & 89.86        & 4       & 91.16        & 99.78        \\
%         Average & 65.586(0.51) & 89.646(0.37) & Average & 91.184(0.06) & 99.804(0.01) \\
%         \bottomrule
%         \label{tab_seed5}
%     \end{tabular}
% \end{table*}

% \subsection{Details of the DLME}

% Manifold nonlinear dimensionality reduction tasks, like t-SNE and UMAP maps the data into 2-D space. 
% Following most manifold learning methods, DLME uses different t-distributions kernel functions in embedding space and semantic space to calculate the pointwise similarity.

% % $\mathcal{S}(x_i,x_j, \nu)=\kappa( d(x_i, x_j), \sigma)=e^{d(x_i,x_j)^2/-\sigma^2}$
% In semantic space:

% \begin{equation*}
%     \begin{aligned}
%     \mathcal{S}_s(x_i,x_j) &= \kappa(d_{j|i} \ | \ \sigma_s,\nu_s) \\
%     &= C_\nu  \left(1+\frac{d_{j|i}^{2}}{\sigma_s \ \nu_s } \right)^{-(\nu_s+1)}, \\
%     \text{with} \ \ C_\nu  &= 2\pi \left(\frac{\Gamma\left(\frac{\nu_s+1}{2}\right)}
%   {\sqrt{\nu_s \pi} \Gamma\left(\frac{\nu_s}{2}\right)}\right)^2
%     \end{aligned}
% \end{equation*}
% where $\sigma_s=1$ for all dataset and $\nu_s=\infty$ (in practice $\nu_s=100$) to let the t-distribution to got to gaussian distribution. $C_\nu$ is a normalizing function satisfying $\lim_{\nu\to +\infty} g(0 \ | \ \sigma, \nu)=1$.

% In embedding space:
% \begin{equation*}
%     \begin{aligned}
%         \mathcal{S}_e(x_i,x_j) &= \kappa(d_{j|i} \ | \ \sigma_e,\nu_e) \\ 
%         &= C_\nu  \left(1+\frac{d_{j|i}^{2}}{\sigma_e \ \nu_e } \right)^{-(\nu_e+1)}, \\ C_\nu  &= 2\pi \left(\frac{\Gamma\left(\frac{\nu_e+1}{2}\right)}
%       {\sqrt{\nu_e \pi} \Gamma\left(\frac{\nu_e}{2}\right)}\right)^2
%     \end{aligned}
% \end{equation*}
% where $\sigma_e=1$ for all dataset and $\nu_e$ is a hyperparameter.



% \subsection{Evaluation Indicators}

% {(1) Accuracy (SVM-ACC)} of a SVM linear classifier trained with the 2-D embedding by 10 fold cross-validation.

% {(2) Continuity (CON)} measures how well the k-NN of a point are preserved when going from the latent to the input space:
% \begin{equation*}
% \begin{aligned}
% \text{CON} &=  1- \mathcal{T}_{\text{CON}}
%       \sum_{i=1}^{|X|} \sum_{j \in \mathcal{N}_{i,k}^{(l)},j \not\in \mathcal{N}_{i,k}^{(l')}}(r^{(l')}_{i,j}-k),\\
%       \mathcal{T}_{CON}&=\frac{2}{|X|k  (2 M-3 k-1)},
% \end{aligned}
% \end{equation*}
% where $\mathcal{T}_{\text{CON}}$ is a normalization term.  $r^{(l')}_{i,j}$ is the rank of $x^{(l')}_j$ in the $k$-NN of $x^{(l')}_i$. $|X|$ is the size of dataset. $\mathcal{N}_{i,k}^{(l')}$ is the set of indices to the $k$-NN of  $x^{(l')}_i$.  $k=|X|/20$.

% \subsection{Data sets and methods}

% % We used 5 datasets (NIST \footnote{https://archive.ics.uci.edu/ml/datasets/Optical+Recognition+of+Handwritten+Digits}, Coil-20 \footnote{https://www.cs.columbia.edu/CAVE/software/softlib/coil-20.php}, Coil-100\footnote{https://www.cs.columbia.edu/CAVE/software/softlib/coil-100.php}, PBMC\footnote{https://support.10xgenomics.com/single-cell-gene-expression/datasets}, Gask-10K\footnote{http://biogps.org/dataset/tag/gastric\%20carcinoma/}) for comparison with 5 methods (UMAP\cite{mcinnes_umap_2018}, t-SNE\cite{maaten_visualizing_2008}, PHATE\cite{moon2019visualizing}, IVIS\cite{szubert_structure-preserving_2019}, P-UMAP\cite{sainburg_parametric_2021}) methods for comparison.
% We use 5 datasets (Mnist \footnote{https://archive.ics.uci.edu/ml/datasets/Optical+Recognition+of+Handwritten+Digits}, Coil-20 \footnote{https://www.cs.columbia.edu/CAVE/software/softlib/coil-20.php}, K-Mnist\footnote{https://www.tensorflow.org/datasets/catalog/kmnist}, PBMC\footnote{https://support.10xgenomics.com/single-cell-gene-expression/datasets}, Gask-10K\footnote{http://biogps.org/dataset/tag/gastric\%20carcinoma/}) and compare with 5 methods (UMAP\cite{mcinnes_umap_2018}, t-SNE\cite{maaten_visualizing_2008}, GRAE\cite{duque2020extendable}, IVIS\cite{szubert_structure-preserving_2019}, P-UMAP\cite{sainburg_parametric_2021}).
% we adopt MLP as the network $g_{\bar \theta}()$ and network $f_{\theta}()$.
% we use the Adamw optimizer with learning rate 0.0001 and weight decay 1e-6. 
% All the models are trained for 4000 epochs. 
% The architecture of $g_{\bar \theta}()$ is [-1, 1000, 800], where -1 mean the dimension of input data. 
% The architecture of $f_{\theta}()$ is [400, 200, 2]. 
% The dimension of embedding space is 2. 
% The hyperparameters and more information of datasets are shown in table \ref{at:5}.

% % \begin{table*}   
% %        \centering
% %        \caption{Hyperparameters of manifold nonlinear dimensionality reduction tasks}
% %        \begin{tabular}{cccccccc}
% %         \hline  
% %          { Dataset }        &  { Point Number }      &  Dimension Number            &  $\nu_e$ &  $M$     &  Batch Size     &  $K$  \\ 
% %         \hline   
% %          { NIST }           &  { 1,797 }             &  { 8$\times$8$\times$1 }     &   0.001  &   100000 &  600            &  5 \\
% %          { Coil20 }         &  { 1,440 }             &  { 128$\times$128$\times$1 } &   0.001  &   100000 &  400            &  5 \\
% %          { Coil100 }        &  { 7,200 }             &  { 128$\times$128$\times$3 } &   0.001  &   100000 &  300            &  5 \\
% %          { PBMC }           &  { 3,000 }             &  { 50 }                      &   0.001  &   100000 &  300            &  5 \\
% %          { Gast-10K }       &  { 10,000 }            &  { 50 }                      &   0.001  &   100000 &  300            &  5 \\
% %         \hline
% %     \end{tabular}
% % \end{table*}



% \section{Experiments Details in Image Representations Tasks}

% CIFAR-10\footnote{https://www.cs.toronto.edu/~kriz/cifar.html}, CIFAR-100\footnote{https://www.cs.toronto.edu/~kriz/cifar.html}, STL-10\footnote{https://cs.stanford.edu/~acoates/stl10/}, tinyImageNet \footnote{https://www.kaggle.com/c/tiny-imagenet} are used in image representation tasks (linear test and image clustering). 
% We we adopt PyTorch to implement BYOL\cite{grill_bootstrap_2020} with ResNet-50 as the encoder architecture and use the Adamw optimizer with learning rate 0.0005 and weight decay 1e-6. 
% We set the temperature $\sigma$ to 1 and the dimension of the latent vector to 256 in all datasets. 
% We use BYOL's data augmentation methods in all datasets and all the models are trained for 400 epochs.
% We set the network $g_{\bar \theta}$ is ResNet-50 and the network $f_{\theta}$ is MLP. 
% As ResNet is designed for images of size 224$\times$224, some previous works modified the standard ResNet and used some tricks (e.g., the Sobel layer used in PICA) to help the network to handle small-sized inputs (e.g., CIFAR-10). 
% The architecture of MLP is:
% \begin{lstlisting}
%     MLP((l1): Linear(in_features=512, out_features=4096, bias=True)
%         (bn1): BatchNorm1d(4096, eps=1e-05, momentum=0.1, 
%                 affine=True, track_running_stats=True)
%         (relu1): ReLU(inplace=True)
%         (l2): Linear(in_features=4096, out_features=256, bias=True))
% \end{lstlisting}

% In both tasks we use a uniform hyperparameter, and the hyperparameter are shown in table \ref{at:6}



% \subsection{Linear test in image representation.}

% Our approach to linear testing comes from BYOL's code\footnote{https://github.com/DonkeyShot21/essential-BYOL}. 
% The data split information is shown in table \ref{at:7}.

% \begin{table*}
%     \centering   
%        \caption{Data indormation of linear test task.}
%        \begin{tabular}{cccccc}
%         \hline \text { Dataset }    & \text { Train data }        & \text { Test data }  & \text { Train Samples } & \text { Test Samples } & \text { Classes } \\
%         \hline \text { CIFAR-10 }   & \text { Train }             & \text { Test }       & 50,000                  & 10,000                 & 10 \\
%         \text { CIFAR-100 }         & \text { Train }             & \text { Test }       & 50,000                  & 10,000                 & 20 \\
%         \text { STL-10 }            & \text { Train + Unlabeled}  & \text { Test }       & 5,000+100,000           & 8,000                  & 10 \\
%         \text { Tiny-ImageNet }     & \text { Train }             & \text { Test }       & 100,000                 & 100,000                & 200 \\
%         \hline
%     \end{tabular}
%     \label{at:7}
% \end{table*}


% \subsection{Image clustering in image representation.}

% For a fair comparison, we use the same experimental setup as linear test and practical the same data divisions as in paper CC\cite{li_contrastive_2020}, which are shown in table\ref{at:8}.




% \section{Visualization of experimental results}

% writing
