# Supplementary material for: DLME: Deep Local-flatness Manifold Embedding
Source: arXiv:2207.03160 source file (2022-07-26)
Supplement: Supplementary file 8 [file Sec_appendix_Results_toy.tex]

\begin{figure}[h]
  \centering
  \includegraphics[width=4in]{fig/FIg-A_SwissRoll.pdf}
  \caption{Training details of TweinSwissRoll dataset}
  \label{fig:appendix_SwissRoll}
\end{figure}

% \begin{figure}[h]
%   \centering
%   \includegraphics[width=5in]{figs/FIg-APPEND_curvature_.pdf}
%   \caption{Visualization comparison with 5 methods on 9 datasets}
%   \label{fig:appendix_vis2}
% \end{figure}

\begin{figure}[h]
  \centering
  \includegraphics[width=4in]{fig/FIg-A_sphere.pdf}
  \caption{Training details of StarFrut dataset}
  \label{fig:appendix_StarFrut}
\end{figure}
